# Supplementary material for: Direct measurement of nonequilibrium system entropy is consistent with Gibbs-Shannon form
Source: arXiv:1703.07601 source file (2017-05-25)
Supplement: Supplementary file 1 [file ShannonSupp.pdf]

# Supplementary Information: Direct measurement of nonequilibrium system entropy is consistent with Gibbs-Shannon form

Momčilo Gavrilov[1,†], Raphaël Chétrite[1,2,3], and John Bechhoefer[1*]
[1] *Department of Physics, Simon Fraser University, Burnaby, British Columbia, V5A 1S6, Canada*
[2] *Pacific Institute for the Mathematical Sciences, UMI 3069, Vancouver, British Columbia, Canada*
[3] *Université Côte d'Azur, CNRS, LJAD, Parc Valrose, 06108 NICE Cedex 02, France*
†*Present address: Department of Biophysics and Biophysical Chemistry, Johns Hopkins University, 725 N. Wolfe Street, Baltimore, MD 21205-2185, USA*

## I. SYSTEM DYNAMICS

The system dynamics are described as one dimensional and overdamped. Here, we give a brief justification for this claim. The inertial damping time of a micron-scale bead in water $\sim \Delta m/\gamma \approx 10^{-6}$ s, where $\Delta m$ is the difference in mass between the bead and the fluid it displaces and where $\gamma$ is the drag coefficient. This time is much shorter than the shortest time scale probed in the experiment, the position-measurement time due to the camera exposure, $\Delta t = 2 \cdot 10^{-4}$ s, and can thus be ignored. The equation of motion is thus a one-dimensional, overdamped Langevin equation of the form given in Eq. 2. Note that the friction coefficient $\gamma$ given there can be calculated from hydrodynamics. For example, for a sphere of radius $a$ moving in an unbounded fluid of viscosity $\eta$, the Stokes solution [1] describing hydrodynamic flow around the sphere implies $\gamma = 6\pi\eta a$. For our case, a sphere near a surface, extra drag due to the surface increases $\gamma$ [1]. The increase in $\gamma$ is apparent through a reduction of the diffusion coefficient, $D = k_\mathrm{B}T/\gamma$. In our case, we observed $D/D_\infty \approx 0.67$, where $D_\infty$ is the value of the diffusion constant predicted using the Stokes drag expression.

Although the particle moves in three-dimensional space, it is confined in two of the dimensions, $y$ and $z$. The motion in $y$ is confined by imposing a virtual potential $U_y(y) \sim \frac{1}{2}k_y y^2$ for deviations from the desired $y$ position. The motion in $z$ is confined by a physical potential that is a balance of electrostatic repulsion between the silica bead and the glass surface and the gravitational attraction. The size and density of the bead are chosen so that the bead is "slightly heavy": it sinks to the bottom but nonetheless fluctuates about an equilibrium height $\approx 0.2$ µm above the glass substrate. Since the $y$ and $z$ dependence of the potential is static, those variables play no role in the thermodynamics, and we can regard the virtual potential as an effectively one-dimensional potential, $U(x,t)$.

* email: johnb@sfu.ca

## II. DERIVATION OF EQ. 10

Starting from $F_{\rm neq}(t) = E(t) - TS(t)$ and writing, as usual, $\beta = (k_{\rm B}T)^{-1}$ to simplify the notation, we have,

$$\begin{aligned}
&(k_{\rm B})^{-1}S(t) + D_{\rm KL}\left(\rho(x,t)\,||\,\rho_{\rm leq}(x,t)\right)\\
&\quad= -\int_{-\infty}^{\infty} \mathrm{d}x\, \rho(x,t)\, \ln \rho(x,t) + \int_{-\infty}^{\infty} \mathrm{d}x\, \rho(x,t)\, \log\left(\frac{\rho(x,t)}{\rho_{\rm leq}(x,t)}\right)\\
&\quad= -\int_{-\infty}^{\infty} \mathrm{d}x\, \rho(x,t)\, \ln \rho_{\rm leq}(x,t)\\
&\quad= -p(t)\int_{-\infty}^{0} \mathrm{d}x\, \rho(x,t|x<0)\, \ln\left[p(t)\, \exp[\beta(F_{\rm leq} - U(x))]\right]\\
&\qquad - (1-p(t))\int_{0}^{\infty} \mathrm{d}x\, \rho(x,t|x>0)\, \ln\left[(1-p(t))\exp[\beta(F_{\rm leq} - U(x))]\right]\\
&\quad= H[p(t)] - p(t)\int_{-\infty}^{0} \mathrm{d}x\, \rho(x,t|x<0)\, [\beta(F_{\rm leq} - U(x))]\\
&\qquad - (1-p(t))\int_{0}^{\infty} \mathrm{d}x\, \rho(x,t|x>0)\, [\beta(F_{\rm leq} - U(x))]\\
&\quad= H[p(t)] - p(t)\beta F_{\rm leq} - (1-p(t))\beta F_{\rm leq}\\
&\qquad + p(t)\beta E(t|x<0) + (1-p(t))\beta E(t|x>0)\\
&\quad= H[p(t)] - \beta[F_{\rm leq} - E(t)]\,.
\end{aligned} \tag{S1}$$

Thus, $TS(t) + k_{\rm B}T\, D_{\rm KL}(\cdot||\cdot) = k_{\rm B}T\, H[p(t)] - F_{\rm leq} + E(t)$, and, finally,

$$\begin{aligned}
F_{\rm neq}(t) &= E(t) - TS(t)\\
&= F_{\rm leq} - k_{\rm B}T\, H[p(t)] + k_{\rm B}T\, D_{\rm KL}\left(\rho(x,t)\,||\,\rho_{\rm leq}(x,t)\right)\,,
\end{aligned} \tag{S2}$$

which is Eq. 10.

Note that the local-equilibrium density function $\rho_{\rm leq}(x,t)$ is discontinuous at $x = 0$ in general for $p \neq \frac{1}{2}$, as illustrated in Fig. S1. It will then be difficult to design a protocol that makes the $D_{\rm KL}$ term vanish at the end. However, if the barrier is high compared to $k_{\rm B}T$, then $\rho_{\rm leq}(x) \approx 0$ in a finite interval about $x = 0$, allowing one to think of the density as approximately two independent conditional densities (Fig. S1a). In such a case, the one chosen for these experiments, it is possible to design a protocol that puts the system in local equilibrium with controllable $p$ at the start and end. The $D_{\rm KL}$ terms then vanish in Eq. 11, making the isolation of the Shannon-entropy contribution to $F_{\rm neq}$ more direct and easier to extract.

## III. A NAIVE VERSION OF PROTOCOL 1

In Figure S2a, we illustrate a naive version of Protocol 1 that is a simple generalization of the protocol used to erase a full bit of information [2]. The system starts with probabilities $p_0$ and $1 - p_0$ for the particle to be in the left and right wells, respectively. At the end, the particle is always in the left well. Then, Eqs. (3) and (4) from the main text imply that the average work should be bounded below by $W \geq k_{\rm B}T(\ln 2)H(p_0)$. Naively, this suggests that, for sufficiently slow protocols, the asymptotic average work will be $W = k_{\rm B}T(\ln 2)H(p_0)$. Instead, we measure $\approx k_{\rm B}T \ln 2$, for all values of $p_0$ (Figure S2b).

Intuitively, we can understand this result using Figure S2c. There, we plot the average work conditioned on whether the particle starts in the left (L) or right (R) wells, $W_{\rm L}$ or $W_{\rm R}$. For large $\tau$ (small $\tau^{-1}$), the plots both converge to $k_{\rm B}T \ln 2$. This makes sense: for slow protocols, the probability density has ample time to mix after the barrier is lowered. Thereafter, the two systems have the same density evolution. And as the barrier is lowered, the symmetry of the system ensures that the contributions to the work from particles starting in either state is the same. Thus, we must have $W_{\rm L} = W_{\rm R}$. But the average work for an initial state occupying the left well with probability $p_0$ can be computed as follows:

$$\begin{aligned}
W &= p_0 W_{\rm L} + (1-p_0)W_{\rm R}\\
&= k_{\rm B}T\left[p_0(\ln 2) + (1-p_0)(\ln 2)\right]\\
&= k_{\rm B}T\, \ln 2\,.
\end{aligned} \tag{S3}$$

Thus, two different lines of reasoning lead to two different lower bounds for the average work to erase. Moreover, the reasoning in both cases suggests that the bounds can be reached by extrapolating slow protocols to the large-

time limit, implying an incompatibility.

To resolve this contradiction, we note that when $p_0 \neq 0.5$, the system is not in global equilibrium. Lowering the barrier is then an irreversible step, because it allows the probabilities to mix. For example, reversing and raising the barrier (immediately after lowering) would lead to a state with probability 0.5 to be in each well, different from the initial state. Because of the dissipation associated with the irreversible mixing of probabilities, the average work must exceed the lower bound of $k_{\rm B}T(\ln 2)\, H(p_0)$ that is derived accounting only for the initial and final states. But why is the average work always $k_{\rm B}T \ln 2$?

To understand this last point more formally, we can use reasoning similar to that of Kawai et al. [3] to derive a refined version of the second law,

$$W \geq \Delta F_{\rm neq} + k_{\rm B}T\, D_{\rm KL}[\rho_{\rm leq}(x,0)||\rho_{\rm eq}(x)]\,, \tag{S4}$$

since the final density of the backward process is the global equilibrium state, $\rho_{\rm eq}(x)$. The relative-entropy term captures the irreversibility of the protocol. An explicit calculation then gives $D_{\rm KL}[\rho_{\rm leq}(x,0)||\rho_{\rm eq}(x)] = p_0 \ln(2p_0) + (1-p_0)\ln[2(1-p_0)] = \ln 2 - H(p_0)$. Since $\Delta F_{\rm neq}/(k_{\rm B}T) = \ln 2$, we have

$$W \geq k_{\rm B}T\, \ln 2\,, \tag{S5}$$

as observed experimentally. In the main text, we see that locally stretching one well to return the initial state to global equilibrium, gives a protocol that does reach the expected thermodynamic bounds.

## IV. DETAILED DEFINITION OF PROTOCOLS 1 AND 2

A protocol is specified by giving a precise definition of the potential $U(x,t)$ in Eq. 15 throughout the protocol, for times $0 \leq t \leq \tau$. In the parametrization of Eq. 15, we need to specify the functions $f(t)$ (tilt), $g(t)$ (barrier height), and $r(t)$ (stretching of the right well). Below, we give the explicit functions for both protocols.

### A. Protocol 1

Protocol 1 is defined by specifying the control functions for tilt, $f_1(t)$, barrier height, $g_2(t)$, and stretching, $r_1(t)$. The coordinate is maximally stretched for $r=1$, where it reaches its full amplitude $\eta$, while no coordinate stretching is present for $r=0$. These three functions are

$$f_1(t) = \begin{cases} (t/\tau - 0.5)/0.25 & t/\tau \in [0.5, 0.75] \\ 1 & t/\tau \in [0.75, 0.85] \\ 1-(t/\tau-0.85)/0.15 & t/\tau \in [0.85, 1] \\ 0 & \text{otherwise} \end{cases} \tag{S6a}$$

$$g_1(t) = \begin{cases} [(t/\tau - 0.5)/0.25]^2 & t/\tau \in [0.25, 0.5] \\ 0 & t/\tau \in [0.5, 0.75] \\ [(t/\tau-0.75)/0.25]^2 & t/\tau \in [0.75, 1] \\ 1 & \text{otherwise} \end{cases} \tag{S6b}$$

$$r(t) = \begin{cases} (t/\tau - 0.25)/0.25 & t/\tau \in [0, 0.25] \\ 1 & t/\tau \in [0.25, 5] \\ 1-(t/\tau-0.5)/0.25 & t/\tau \in [0.5, 0.75] \\ 0 & \text{otherwise} \end{cases}. \tag{S6c}$$

### B. Protocol 2

Protocol 2 does not involve stretching, meaning that $r_2(t) = 1$ for all time. The control functions for tilt and barrier height are given by

$$f_2(t) = \begin{cases} (t/\tau - 0.5)/0.25 & t/\tau \in [0.5, 0.75] \\ 1 & t/\tau \in [0.75, 0.85] \\ 1-(t/\tau-0.85)/0.15 & t/\tau \in [0.85, 1] \\ 0 & \text{otherwise} \end{cases} \tag{S7a}$$

$$g_2(t) = \begin{cases} [(t/\tau - 0.5)/0.5]^2 & t/\tau \in [0, 1] \\ 1 & \text{otherwise} \end{cases}. \tag{S7b}$$

## V. CONDITIONED FLUCTUATION RELATION AND ASYMPTOTIC WORK FROM FINITE-TIME MEASUREMENTS IN PROTOCOL 2: THEORY

Starting from the seminal work of Jarzynski [4], one theme of stochastic thermodynamics is that it is possible to estimate equilibrium thermodynamic quantities such as equilibrium free-energy differences from measurements that are conducted on systems out of thermodynamic equilibrium. In this section, we will consider analogous ways to estimate differences in *nonequilibrium* free energies for states that are in local equilibrium, as defined in Eq. 8.

In Protocol 2, we consider a finite time protocol that starts from a full bit and erases it partially using a tilt in

the trajectory. For fixed tilt magnitude, the probability $p_\tau$ to be in the left well at time $\tau$ depends on $\tau$ in a way not known analytically a priori. Moreover, empirical extrapolation to the asymptotic occupation probability, $\lim_{\tau\to\infty} p_\tau$, is not accurate enough, as the uncertainties in estimated probabilities increase with the cycle time $\tau$. (Longer cycle times leads to fewer repetitions.) Thus, we cannot extrapolate to infinite $\tau$, as we did in Protocol 1.

To estimate asymptotic work using Protocol 2 therefore requires a different strategy that works with measurements performed at a single (large) value of $\tau$. Here, we show that by measuring first the average work to carry out the finite-time protocol and then the average work to carry out a time-reversed version of the same protocol, we can deduce the asymptotic minimal average work, $W = W_\infty$, i.e., $\Delta F_{\text{neq}}$ in Eq. 4 of the main text.

### A. Conditioned fluctuation relation

We start by defining some notation. Let $P_{\text{F}}(x_0, x_\tau, w)$ be the joint probability for a realization of the forward experiment where a particle starts at position $x_0$ at time $t = 0$ and finishes at position $x_\tau$ at time $t = \tau$ and for which the changing potential exerts a stochastic work $w$ on the particle. To be more explicit, consider a path integral over all trajectories $[x]_0^\tau$ from 0 to $\tau$ with fixed endpoints and work,

$$P_{\text{F}}(x_0, x_\tau, w) = \int \mathcal{D}x \, P_{\text{F}}([x]_0^\tau) \times \left[\delta(x(0) - x_0)\, \delta(x(\tau) - x_\tau)\, \delta(w([x]_0^\tau) - w)\right] , \tag{S8}$$

where $P_{\text{F}}([x]_0^\tau)$ is the probability of the path $[x]_0^\tau$ and where $w([x]_0^\tau)$ is the work associated with a given trajectory $[x]_0^\tau$ (Eq. 16).

Next, assume that the system starts in global equilibrium, which, in the context of this experiment, implies that the system is in local equilibrium within each well, with equal probabilities to be in the two macrostates. The density corresponds to $\rho_{\text{leq}}(x, t)$ in Eq. 8, with $p(t) = \frac{1}{2}$, which we denote $\rho_{\text{eq}}(x)$.

For the backward protocol defined by $U_{\text{B}}(x, t) = U(x, \tau - t)$, we analogously define the probability $P_{\text{B}}(x_\tau, x_0, -w)$ that the particle starts at time $t = 0$ at position $x_\tau$, ends at time $t = \tau$ at position $x_0$, and the potential exerts a work $-w$ on the particle. We further assume that the initial density of the backward protocol is chosen to be the global equilibrium. In the experimental Protocol 2 described in the Methods, the fact that the backward part of the protocol immediately follows the forward part means that the initial density is actually different—local equilibrium with probability $p_\tau$ for the left well—but this difference turns out not to affect the conditional fluctuation relations that we derive below.

We can relate $P_{\text{F}}(x_0, x_\tau, w)$ to $P_{\text{B}}(x_\tau, x_0, -w)$ using the Detailed Fluctuation Relation [5, 6], which generalizes the detailed-balance condition of equilibrium to nonequilibrium situations. Because the protocol is cyclic, with $U(x, 0) = U(x, \tau)$, the usual equilibrium free-energy difference vanishes, and the relation takes a simple form:

$$P_{\text{B}}(x_\tau, x_0, -w) = \mathrm{e}^{-\beta w}\, P_{\text{F}}(x_0, x_\tau, w) \, . \tag{S9}$$

We next marginalize over initial and final positions by integrating $x_0$ over $(-\infty, \infty)$ and $x_\tau$ over $(-\infty, 0)$, thereby isolating forward trajectories that end in the left well (state $L$). Imposing in Eq. S9 initial conditioning for the left-hand side and final conditioning for the right-hand side, we then obtain,

$$\underbrace{\left(\int_{-\infty}^{0} \mathrm{d}x \, \rho_{\text{eq}}(x)\right)}_{1/2} P_{\text{B|L}}(-w) = \mathrm{e}^{-\beta w} \underbrace{\left(\int_{-\infty}^{0} \mathrm{d}x \, \rho_{\text{leq}}(x)\right)}_{p_\tau} P_{\text{F|L}}(w) \, , \tag{S10}$$

where $P_{\text{F|L}}(w)$ is the conditional probability to start in global equilibrium, *finish* in $L$, and exert work $w$ in the forward protocol and where $P_{\text{B|L}}(-w)$ is the conditional probability to *start* in $L$ and exert work $-w$ in the backward protocol.

Alternatively, we could have integrated over the $R$ state ($x > 0$) at $t = \tau$, to find

$$\underbrace{\left(\int_{0}^{\infty} \mathrm{d}x \, \rho_{\text{eq}}(x)\right)}_{1/2} P_{\text{B|R}}(-w) = \mathrm{e}^{-\beta w} \underbrace{\left(\int_{0}^{\infty} \mathrm{d}x \, \rho_{\text{leq}}(x)\right)}_{1-p_\tau} P_{\text{F|R}}(w) \, , \tag{S11}$$

where, in our slow protocol, the forward process finishes at time $\tau$ in local equilibrium $\rho_{\text{leq}}$.

Thus, we have the "conditioned Crooks" relations,

$$P_{\text{B|L}}(-w) = 2p_\tau \, \mathrm{e}^{-\beta w}\, P_{\text{F|L}}(w) \tag{S12a}$$

$$P_{\text{B|R}}(-w) = 2(1 - p_\tau)\, \mathrm{e}^{-\beta w}\, P_{\text{F|R}}(w) \, . \tag{S12b}$$

A crucial point for us is that, because of the initial conditioning, $P_{\text{B|L}}(-w)$ is identical regardless of whether the backward protocol starts in global equilibrium or in a local equilibrium with arbitrary $p_\tau$. Thus, even though we suppose in the Detailed Fluctuation Relation, Eq. S9, that the backward system starts in global equilibrium, Eq. S12a is valid for the backward protocol used in our Protocol 2. Similar statements apply to $P_{\text{B|R}}(-w)$ and Eq. S12b.

If we integrate the conditional Crooks relations in Eq. S12a and b with respect to work, we find the condi-

tional Jarzynski relations,

$$\left\langle \mathrm{e}^{-w/k_\mathrm{B}T} \right\rangle_{\mathrm{F|L}} = \frac{1}{2p_\tau} \tag{S13a}$$
$$\left\langle \mathrm{e}^{-w/k_\mathrm{B}T} \right\rangle_{\mathrm{F|R}} = \frac{1}{2(1-p_\tau)} \,. \tag{S13b}$$

By Jensen's inequality, we then obtain refinements of the second law in two "conditioned" forms,

$$W_{\mathrm{F|L}} \geq k_\mathrm{B}T \ln\left(2p_\tau\right) \tag{S14a}$$
$$W_{\mathrm{F|R}} \geq k_\mathrm{B}T \ln\left(2\left(1-p_\tau\right)\right) \,. \tag{S14b}$$

Analogous relations were experimentally verified in the context of breaking or restoring ergodicity in [7].

Our protocol can be interpreted in the framework of thermodynamics of symmetry breaking and symmetry restoration of Ref.[7]. The first part of the protocol can be interpreted as a symmetry restoration (see the conditioned second principle given in Eq. S.15 of [7], with $p_i \to 1/2$) followed by a symmetry breaking (Eq. S.7 of [7] with $p_i \to p_\tau$). By summing these two relations, the equilibrium free energy difference disappears, and we find Eq. S14a (and similarly for Eq. S14b). In Section VI B, we will see that we can also interpret the results of our experiments as testing the conditioned Crooks relation, Eq. S12, directly.

### B. Conditionally Gaussian work fluctuations

We are now interested in the case where the forward and backward conditional probability density functions are Gaussian distributions, as is the case experimentally for slow protocols. Note that in this case, the unconditioned work is not Gaussian but is rather the weighted sum of Gaussians. This fact traces back to the observation that the protocol time $\tau$ is long enough to reach local equilibrium but short with respect to global equilibrium, which would be achieved by hops over the barrier. Under these assumptions, we can write Eq. S12a as

$$\frac{\exp\left(-\frac{(w+W_{\mathrm{B|L}})^2}{2\sigma^2_{\mathrm{B|L}}}\right)}{\sqrt{2\pi\sigma^2_{\mathrm{B|L}}}} = 2\,\mathrm{e}^{-\beta w}\, p_\tau \frac{\exp\left(-\frac{(w-W_{\mathrm{F|L}})^2}{2\sigma^2_{\mathrm{F|L}}}\right)}{\sqrt{2\pi\sigma^2_{\mathrm{F|L}}}} \,. \tag{S15}$$

Rearranging terms gives

$$\exp\left(-\frac{(w-W_{\mathrm{F|L}})^2}{2\sigma^2_{\mathrm{F|L}}} + \frac{(w+W_{\mathrm{B|L}})^2}{2\sigma^2_{\mathrm{B|L}}} - \beta w + \ln(2p_\tau)\right) = \frac{\sigma_{\mathrm{F|L}}}{\sigma_{\mathrm{B|L}}} \,. \tag{S16}$$

Taking a natural logarithm and isolating terms of the same order in $w$ gives

$$w^2\left[-\frac{1}{2\sigma^2_{\mathrm{F|L}}} + \frac{1}{2\sigma^2_{\mathrm{B|L}}}\right] + w\left[\frac{W_{\mathrm{F|L}}}{\sigma^2_{\mathrm{F|L}}} + \frac{W_{\mathrm{B|L}}}{\sigma^2_{\mathrm{B|L}}} - \beta\right] + \left[-\frac{W^2_{\mathrm{F|L}}}{2\sigma^2_{\mathrm{F|L}}} + \frac{W^2_{\mathrm{B|L}}}{2\sigma^2_{\mathrm{B|L}}} + \ln(2p_\tau)\right] = \ln\left(\frac{\sigma_{\mathrm{F|L}}}{\sigma_{\mathrm{B|L}}}\right) \,. \tag{S17}$$

Since Eq. S17 must hold for all values of $w$, the prefactors of $w^2$ and $w$, as well as the constant terms, must each vanish separately. For $w^2$, we conclude that

$$\sigma_{\mathrm{F|L}} = \sigma_{\mathrm{B|L}} \equiv \sigma_\mathrm{L} \,. \tag{S18}$$

The $w$ and constant terms then imply

$$W_{\mathrm{F|L}} + W_{\mathrm{B|L}} = \beta\sigma^2_L \tag{S19a}$$
$$W^2_{\mathrm{F|L}} - W^2_{\mathrm{B|L}} = 2\sigma^2_L \ln(2p_\tau) \,. \tag{S19b}$$

From the ratio of Eq. S19b to Eq. S19a, we deduce that

$$W_{\mathrm{F|L}} + W_{\mathrm{B|L}} = \beta\sigma^2_L \tag{S20a}$$
$$W_{\mathrm{F|L}} - W_{\mathrm{B|L}} = \tfrac{2}{\beta}\ln(2p_\tau) \,. \tag{S20b}$$

Adding and subtracting Eqs. (S20a) and (S20b) gives

$$W_{\mathrm{F|L}} = \tfrac{\beta}{2}\sigma^2_L + \tfrac{1}{\beta}\ln(2p_\tau) \tag{S21a}$$
$$W_{\mathrm{B|L}} = \tfrac{\beta}{2}\sigma^2_L - \tfrac{1}{\beta}\ln(2p_\tau) \,. \tag{S21b}$$

A similar argument conditioned on the $R$ state gives

$$W_{\mathrm{F|R}} = \tfrac{\beta}{2}\sigma^2_R + \tfrac{1}{\beta}\ln(2(1-p_\tau)) \tag{S22a}$$
$$W_{\mathrm{B|R}} = \tfrac{\beta}{2}\sigma^2_R - \tfrac{1}{\beta}\ln(2(1-p_\tau)) \,. \tag{S22b}$$

Now, by using the law of total probability, we can obtain the average unconditioned forward work $W_\mathrm{F}$ and the average unconditioned backward work $W_\mathrm{B}$. In Protocol 2, the forward process finishes in local equilibrium. The backward process starts in the same local-equilibrium state, and we obtain

$$W_\mathrm{F} = p_\tau\, W_{\mathrm{F|L}} + (1-p_\tau)\, W_{\mathrm{F|R}} \tag{S23a}$$
$$W_\mathrm{B} = p_\tau\, W_{\mathrm{B|L}} + (1-p_\tau)\, W_{\mathrm{B|R}} \,. \tag{S23b}$$

Finally, from Eqs. (S21)–(S23), we have

$$\begin{aligned}\tfrac{1}{2}\left(W_\mathrm{F} - W_\mathrm{B}\right) &= \tfrac{1}{2}p_\tau\left(W_{\mathrm{F|L}} - W_{\mathrm{B|L}}\right) \\ &\quad + \tfrac{1}{2}(1-p_\tau)\left(W_{\mathrm{F|R}} - W_{\mathrm{B|R}}\right) \\ &= \tfrac{1}{\beta}\left[p_\tau \ln(2p_\tau) + (1-p_\tau)\ln(2(1-p_\tau))\right] \\ &= k_\mathrm{B}T\,(\ln 2)\left[1 - H(p_\tau)\right] ,\end{aligned} \tag{S24}$$

which is Eq. 14 in the main text, with $H(p_\tau)$ in bits. Here, Eq. S24 is valid for states that are in local equilibrium, as defined in Eq. 8.

Thus, by a careful combination of the easily measured average quantities $W_{\mathrm{F}}$ and $W_{\mathrm{B}}$ from the forward and backward protocols, the terms involving the variances $\sigma_{\mathrm{L}}^2$ and $\sigma_{\mathrm{R}}^2$ cancel, and we can isolate the desired Shannon-entropy term $H(p_\tau)$. Intuitively, the average work done is composed of two terms: one from the asymptotic nonequilibrium free energy and one from the fluctuations due to a finite-time protocol. Because of the even character of fluctuations at finite time, half the difference of $W_{\mathrm{F}}$ and $W_{\mathrm{B}}$ then corresponds to averaging the nonequilibrium free energy contribution while canceling the dissipation due to a finite-time protocol. We stress that this cancelation works, in general, only for slow protocols where conditional distributions are Gaussian (but no hops over the barrier occur).

## VI. CONDITIONED FLUCTUATION RELATION AND ASYMPTOTIC WORK FROM FINITE-TIME MEASUREMENTS IN PROTOCOL 2: EXPERIMENT

Protocol 2 begins with one bit of information, with the initial probability to be in the left state $p_0 = \frac{1}{2}$, and erases a fraction of the information by altering the probability at the end of the protocol to $p_\tau$, which is in the range $0 \leq p_\tau \leq 1$. Tilting the double-well potential by a small amount would seem a straightforward way to erase a small amount of information. Unfortunately, predicting the tilt needed to bring two states to equilibrium when crossover (mixing) occurs is difficult. Since the crossover time also depends on the rate at which the barrier is lowered, the required tilt varies with cycle time. But varying the tilt also alters $p_\tau$, which must then also be extrapolated to long times. These onerous requirements rule out extrapolation as a practical way of measuring the mean work in a protocol with tilt. As a way around this difficulty, we designed Protocol 2 with a small tilt, but we work at a fixed protocol time $\tau$. To isolate the minimal average work, we combine both forward and backward manipulations of the potential and use the results derived above in Section V.

Protocol 2 is illustrated in Fig. S3. The first step is to lower the barrier. The next is to tilt the potential by the chosen amplitude, $A$. Positive tilt amplitudes ($A > 0$) tend to push the particle to the right and decrease the probability $p_\tau$ to end up in the *left* well at time $\tau$. The last step in the forward part of the protocol is to restore the barrier to the original height of 10 $k_{\mathrm{B}}T$ and untilt.

Figure S4 shows the probability $p_\tau$ that the system ends up in the left well at time $\tau$ as a function of tilt amplitude $A$ (red markers). We note that, for fixed $A$, the probability at the end of the protocol depends on its length $\tau$. The results presented here and in the main text are all for $\tau = 2$. Recall that the cycle time $\tau$ is scaled by $\tau_0 = (2x_m)^2/D \approx 10$ s, which is the time for a particle to diffuse the distance between the two local minima, in the absence of a virtual potential. At the end of the forward part of the protocol, we reverse the changes in the potential. The gray markers in Figure S4 confirm that the protocol is reversible: for all tilt amplitudes $A$, the system returns to its initial state with $p_0 = 0.5$, and $H_0 = 1$. We estimate work using Sekimoto's formula for both the forward and time-reversed protocol sections. (See Methods, Eq. 16.)

In the main text, we assert that we can deduce the form of the Gibbs-Shannon entropy function via measurements of the mean work to carry the forward and backward portions of the protocol (Eq. 5 of the main text), as derived above in Section V B. That derivation assumes, first of all, that conditional work distributions are Gaussian. It also uses intermediate results such as the conditioned Crooks relations, Eq. S12. Here, we give experimental evidence to support these claims and assumptions.

### A. Experimental conditional work distributions are consistent with Gaussian

We begin by showing that the conditional work distributions are consistent with the Gaussian form. Figure S5a shows the measured work distributions for the forward $P_{\mathrm{F}}(w)$ and backward $P_{\mathrm{B}}(-w)$ protocols. Although difficult to see explicitly given our resolution, these are *not* expected to be Gaussian but are rather the sum of two conditional Gaussian distributions, depending on whether the particle ends up in the left or right wells (forward protocol) or starts in one of those states (reverse protocol). The solid lines denote the sum of two Gaussian fits to conditional distributions, weighted by the probability for the forward protocol to end up in the left well.

We next use the law of total probability to decompose the work distributions into conditional distributions for a particle ending (or starting) in either well:

$$P_{\mathrm{F}}(w) = p_\tau P_{\mathrm{F|L}}(w) + (1-p_\tau) P_{\mathrm{F|R}}(w) \tag{S25a}$$

$$P_{\mathrm{B}}(-w) = p_\tau P_{\mathrm{B|L}}(-w) + (1-p_\tau) P_{\mathrm{B|R}}(-w)\,, \tag{S25b}$$

where $P_{\mathrm{F|L}}(w)$, $P_{\mathrm{F|R}}(w)$, $P_{\mathrm{B|L}}(-w)$, and $P_{\mathrm{B|R}}(-w)$ are defined in Section V A. Figure S5b and c shows the histogram estimates of the conditional work distributions. The solid lines show that the protocols are slow enough that the empirical conditional work distributions are consistent with Gaussian distributions.

Finally, Figure S6 compares $W_{\mathrm{F}}$, $W_{\mathrm{B}}$, and $H(p_\tau)$. We stress that the protocols must be executed sufficiently slowly that the conditional work distributions are Gaussian.

### B. Experimental test of conditional Crooks relations

The next step is to show that our experimental results are consistent with the conditional Crooks relations,

Eq. S12. Similar tests have been previously done by Junier et al. [8]. First, we plot the measured conditional work distributions for the backward protocols, $P_{\mathrm{B|L}}(-w)$ and $P_{\mathrm{B|R}}(-w)$, along with their Gaussian fits. These are the red markers and light red solid line in Fig. S7a and b and reproduce the results of Fig. S5. We then calculate the corresponding forward conditional work distributions $P_{\mathrm{F|L}}(w)$ and $P_{\mathrm{F|R}}(w)$ using Eq. S12 and plot that distribution as the light black curves in Fig. S7a and b. Finally, we plot the measured conditional work distributions and show that they are consistent with values expected. The agreement is tested to a higher precision for a particle ending in the left well (Fig. S7a), because the probability for ending in the left well is $p_\tau = 0.85 \pm 0.02$, which implies that there are more work measurements for a particle ending in the left well and, hence, better statistics. In brief, we have shown that the two conditional distributions are related as the conditional Crooks relation asserts they should be.

To test these relations in another way, we sum Eq. S12 and combine with Eq. S25 to find

$$\ln\left(\frac{2P_{\mathrm{F}}(w)}{P_{\mathrm{B|L}}(-w)+P_{\mathrm{B|R}}(-w)}\right) = \frac{w}{k_{\mathrm{B}}T}\,. \tag{S26}$$

In Fig. S7c, we plot the left-hand side of Eq. S26 versus work $w$ (red markers) and confirm the expected linear relation (solid line).

## VII. TESTING THE CONTINUUM VERSION OF THE SHANNON ENTROPY FUNCTION

In the main text, we show experimentally that the system entropy $S$ that appears in the second law (Eq. 3) is consistent with the Gibbs-Shannon form of the entropy (Eq. 1). In fact, our experiment also tests a stronger statement: In the Markovian context of Langevin equations such as Eq. 2, the total entropy production $S_{\mathrm{tot}}$ that appears in Eq. 3 of the main text is equal to [6, 9, 10],

$$S_{\mathrm{tot}} = D_{\mathrm{KL}}\left(P_{\mathrm{F}}\left([x]_0^\tau\right) \mid P_{\mathrm{B}}\left(\overleftarrow{[x]_0^\tau}\right)\right)\,, \tag{S27}$$

where $P_{\mathrm{F}}\left([x]_0^\tau\right)$ is the probability of the path $[x]_0^\tau$ under the forward protocol and $P_{\mathrm{B}}\left(\overleftarrow{[x]_0^\tau}\right)$ is the probability of the same path $[x]_0^\tau$, but read backward, for the backward protocol based on the potential $U^{\mathrm{B}}(x,t) = U(x,\tau - t)$. The initial density of the backward process is $\rho(x,\tau)$.

More precisely, after defining the form of the work $W$ done on the system to be the average of the Sekimoto formula (Eq. 16), we can use the first law (Eq. 4 of the main text) to deduce the form of the heat $Q$ exchanged with the medium. The Clausius relation then implies the associated form of the exchanged entropy $S_{\mathrm{m}}$ that appears in Eq. 3. We can then prove, using Eq. 3 of the main text, that the Gibbs-Shannon form for $S$ is equivalent to the form of $S_{\mathrm{tot}}$ given here in Eq. (S27) [6].

Finally, those who consider it "obvious" to use the Gibbs-Shannon form of entropy in the second law (Eq. 3) will perhaps agree that testing the form of $S_{\mathrm{tot}}$ given in Eq. S27 is less obvious.


[1] J. Happel and H. Brenner, *Low Reynolds Number Hydrodynamics: With Special Applications to Particulate Media* (Martinus Nijhoff, 1983).

[2] Y. Jun, M. Gavrilov, and J. Bechhoefer, "High-precision test of Landauer's principle in a feedback trap," Phys. Rev. Lett. **113**, 190601 (2014).

[3] R. Kawai, J. M. R. Parrondo, and C. Van den Broeck, "Dissipation: The phase-space perspective," Phys. Rev. Lett. **98**, 080602 (2007).

[4] C. Jarzynski, "Nonequilibrium equality for free energy differences," Phys. Rev. Lett. **78**, 2690–2693 (1997).

[5] C. Jarzynski, "Hamiltonian derivation of a detailed fluctuation theorem," J. Stat. Phys. **98**, 77–102 (2000).

[6] R. Chétrite and K. Gawędzki, "Fluctuation relations for diffusion processes," Commun. Math. Phys. **282**, 469–518 (2008).

[7] É. Roldán, I. A. Martínez, J. M. R. Parrondo, and D. Petrov, "Universal features in the energetics of symmetry breaking," Nature Phys. **10**, 457–461 (2014).

[8] I. Junier, A. Mossa, M. Manosas, and F. Ritort, "Recovery of free energy branches in single molecule experiments," Phys. Rev. Lett. **102**, 070602 (2009).

[9] C. Maes and K. Netočný, "Time-reversal and entropy," J. Stat. Phys. **110**, 269–310 (2003).

[10] C. Maes, "The fluctuation theorem as a Gibbs property," J. Stat. Phys. **95**, 367–392 (1999).

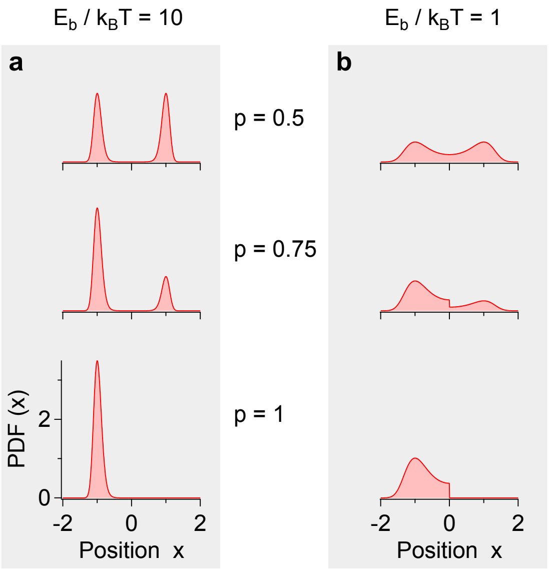


FIG. S1. Effect of dimensionless barrier height $E_\mathrm{b}/k_\mathrm{B}T$ on local equilibrium distribution, $\rho_\mathrm{leq}(x)$ for a symmetric, double-well potential. **a**, For a high barrier, there are effectively two separate distributions for all weights $p(t)$. **b**, For a low barrier, there is a significant jump discontinuity in density at $x = 0$ for $p(t)$ sufficiently different from 0.5.

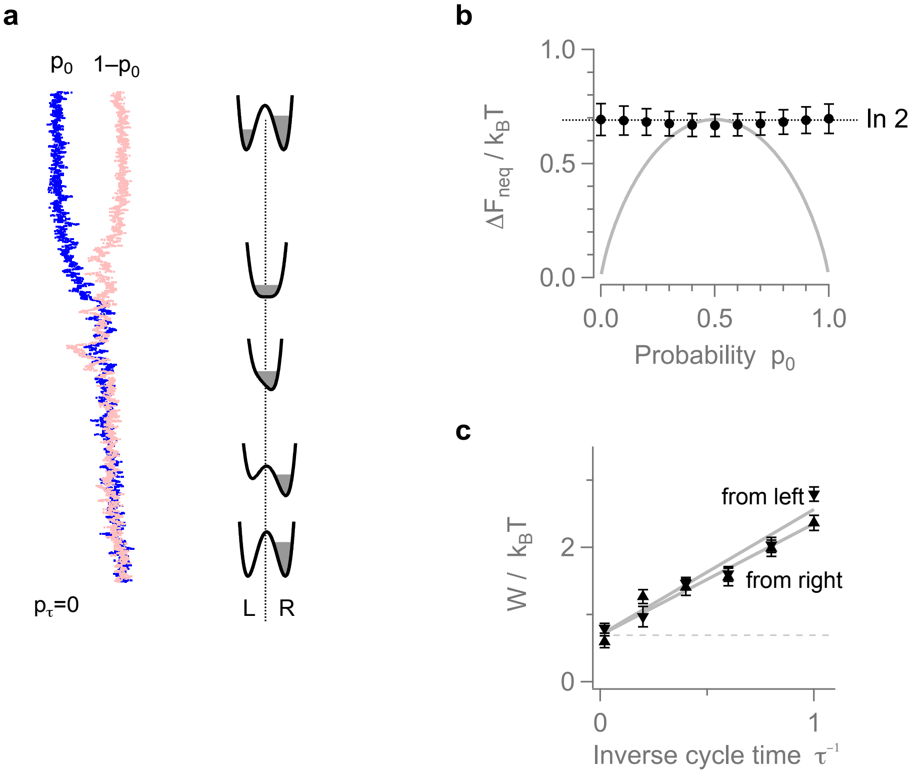


FIG. S2. Naive version of Protocol 1. **a**, Sample trajectories starting from left and right wells, along with potentials at time points within the protocol. **b**, For all initial probabilities $p_0$, the average change in nonequilibrium free energy to erase is $k_\mathrm{B}T \ln 2$ for slow protocols. **c**, The average conditional work to erase is asymptotically $k_\mathrm{B}T \ln 2$ for particles that start in the left well and also for particles that start in the right well.

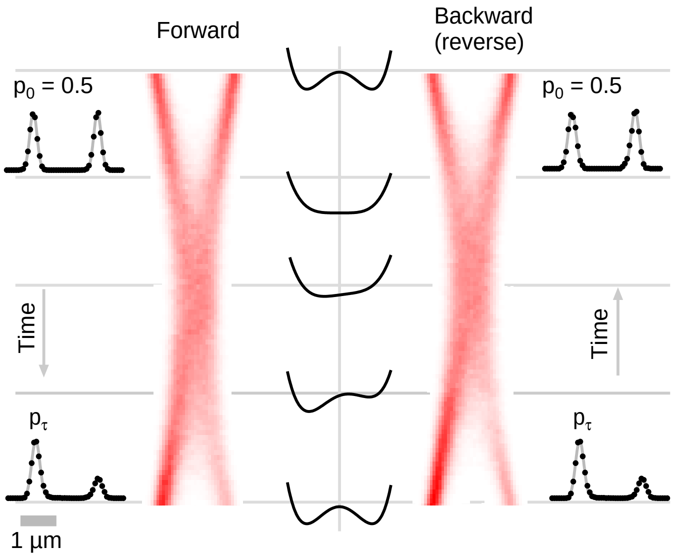


FIG. S3. Protocol 2: Path probability densities for partial erasure in the forward protocol (left) and its accompanying backward protocol (right). In the forward protocol, one bit of information is erased to the left well, with probability $p_\tau = 0.75 \pm 0.02$ for tilt amplitude $A = -0.03$. The duration of the protocol, $\tau = 2$, corresponds to a physical time of 20 s. The backward protocol, played forward in time, returns a particle to the initial state with probability 0.5.

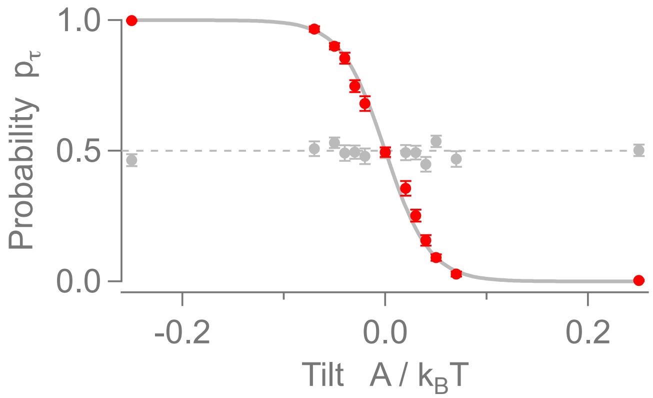


FIG. S4. Erasure probability recorded for different tilt amplitudes. Red markers show probability $p_\tau$ at the end of the partial erasure experiment, while gray markers show the probability of ending up in the left well for the time-reversed protocol. Solid gray line is empirical function relating the tilt amplitude $A$ to the probability $p_\tau$ of being in the $L$ state at time $\tau$, given by $p_\tau = f(A) = 0.5[1 - \tanh(23A)]$ for $\tau = 2$.

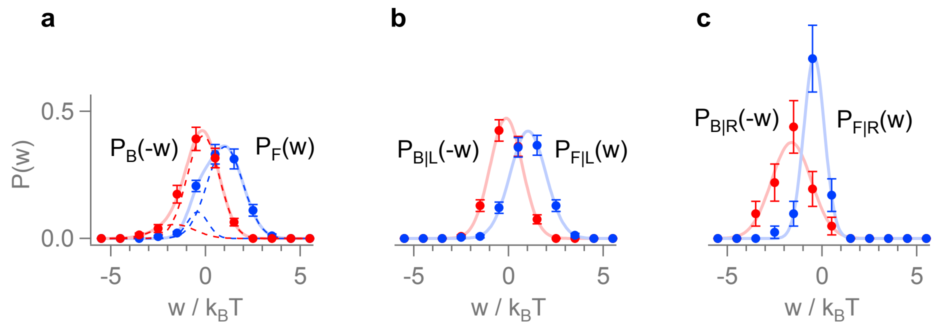


FIG. S5. Conditional work distributions are consistent with Gaussian. **a**, Estimated unconditioned work distributions $P_{\mathrm{F}}(w)$ and $P_{\mathrm{B}}(-w)$ for forward and reverse parts of protocols (red and blue markers). Solid lines represent the sum of the corresponding two Gaussian distributions in b and c. Dashed lines show contributions from weighted conditional Gaussian distributions. **b**, Conditional work distributions for the left state for forward $P_{\mathrm{F|L}}(w)$ and backward $P_{\mathrm{B|L}}(-w)$ protocols. Solid lines are fits to Gaussian distributions. **c**, Same, for right state. Tilt amplitude is set to $A/k_{\mathrm{B}}T = -0.04$, and we measure $p_\tau = 0.85 \pm 0.02$.

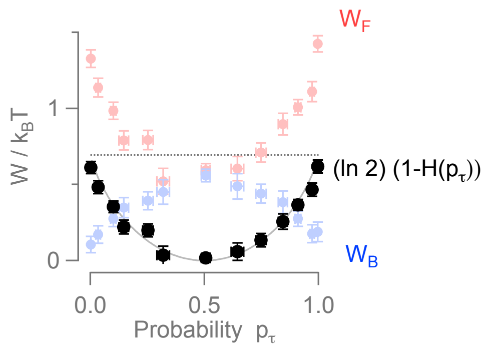


FIG. S6. Mean work in forward protocol $W_{\mathrm{F}}$ compared with reverse protocol $W_{\mathrm{B}}$. The desired Shannon-entropy term $H(p_\tau)$ is isolated from $W_{\mathrm{F}}$ and $W_{\mathrm{B}}$ using Eq. 14 of the main text, or Eq. S24 here.

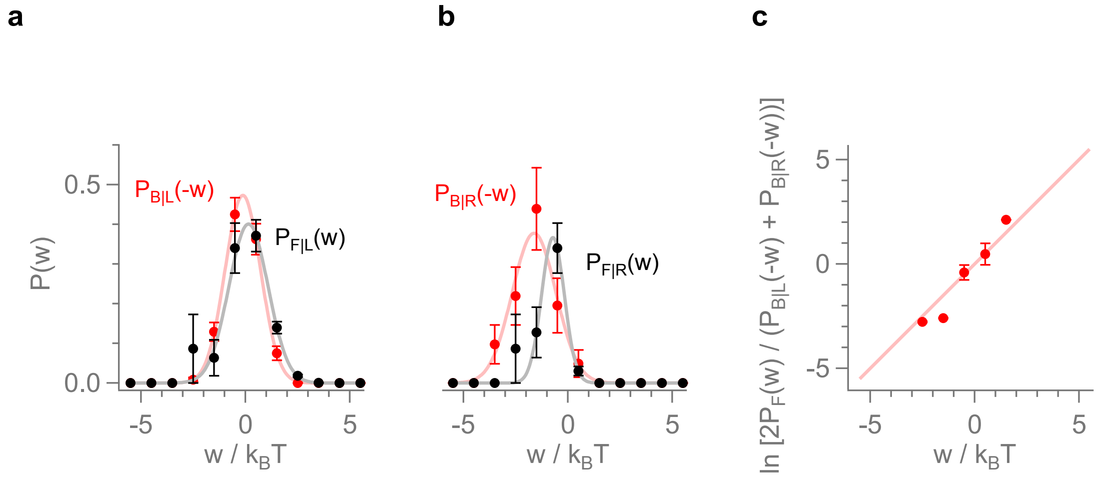


FIG. S7. Comparison between measured and calculated conditional work distributions for Protocol 2. **a**, Conditional work distribution with left-well conditioning. Red markers show measured values, black markers shows estimates using Eq. S12a. **b**, Conditional work distribution with right-well condtioning. Red markers show measured values, black markers shows estimates using Eq. S12b. **c**, Test of Eq. S26. Solid line has slope = 1.
